# Supplementary material for: Superconductivity in the dilute single band limit in reduced Strontium Titanate
Source: arXiv:1904.03121 source file (2019-09-30)
Supplement: Supplementary file 1 [file Low_n_SC_Supplemental_Material_v27_compressed.pdf]

## Supplemental Material:

## *Superconductivity in the dilute single band limit in reduced Strontium Titanate*

Terence M. Bretz-Sullivan,[1] Alexander Edelman,[2] J. S. Jiang,[1] Alexey Suslov,[3] David Graf,[3] Jianjie Zhang,[4] Gensheng Wang,[4] Clarence Chang,[2,4] John E. Pearson,[1] Alex B. Martinson,[1] Peter B. Littlewood[1,2] and Anand Bhattacharya[1]

[1] *Materials Science Division, Argonne National Laboratory, 9700 S. Cass Avenue, Lemont, IL 60439*
[2] *Department of Physics, The University of Chicago, 5720 South Ellis Avenue, Chicago, IL 60637*
[3] *The National High Magnetic Field Laboratory, 1800 E. Paul Dirac Drive, Tallahassee, FL 32310*
[4] *High Energy Physics Division, Argonne National Laboratory, 9700 S. Cass Avenue, Lemont, IL 60439*

**Table of contents:** **pg.**

Section 1: Sample preparation details…………………………………………………………………….2

Section 2: Cryostat and electrical transport details……………………………………………………2

Section 3: Electrical transport results for samples A-F……………………………………………...4

Section 4: Tunnel diode oscillator (TDO) results…………………………………………………..…8

Section 5: Computed length and energy scales, estimates of the depairing currents…….9

Section 6: Paraconductivity, EMT fits and theoretical discussions……………………………...10

Section 7: Superconducting transitions for samples G-J (measured along [011])………….15

## Section 1: Sample preparation details

**Rocking curves:** We obtained atomically smooth, one side polished undoped 10mm x 10mm x 0.5mm (100) $SrTiO_3$ single crystal substrates from CrysTec Gmbh. We vetted all samples for crystallinity using X-ray diffraction using Cu-$K_\alpha$ radiation. The rocking curve of the $SrTiO_3$ (200) reflection had a full width at half maximum (Δω) in the range of $0.020^\circ < \Delta\omega < 0.066^\circ$ for all the measured samples. In Fig. S1 are the measured rocking curves for samples A-F.

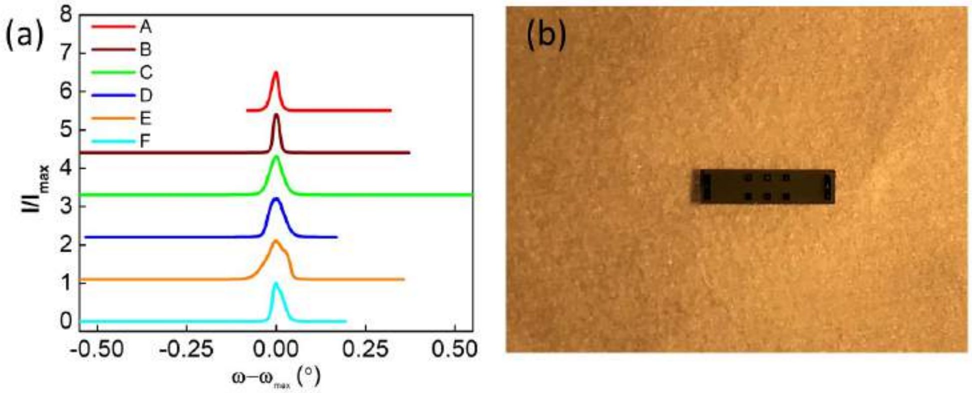


**Fig. S1**. (a) Rocking curves of the as-received substrates. The curves are offset for clarity. (b) An optical micrograph of sample C with dimensions 10 x 2.5 x 0.5 mm.

**Annealing procedure:** To introduce dopants, oxygen vacancies, into the STO substrates, we followed an annealing procedure as previously done by our group. We heated the substrates at 20° C/min to 625°C-750°C and annealed for 60 minutes. At the end of the annealing step, we turned off the heater and allowed the sample to cool down in vacuum to room temperature.

**Device fabrication:** After the annealing step, we used photolithography to pattern the contact pads. We then $Ar^+$ ion milled, at $V_{beam}$ = 300 V, $V_{acc}$ = 100 V and 45° incidence, the contact areas for 15 minutes and sputtered Ti/Au contacts of thicknesses 20 nm/80 nm in a Hall bar geometry. Samples A-F had dimensions $(L, W, H)$ of 10 mm x 2.5 mm x 0.5 mm. Samples G-J had dimensions 5 mm x 5 mm x 0.5 mm. An optical micrograph of sample C in in Fig. S1 (b).

## Section 2: Cryostat and electrical transport details

**PPMS, dilution refrigerators and measurement electronics:** We carried out our measurements in several dilution fridges, including (i) a Quantum Design Physical Property Measurement System with a 14T superconducting magnet (PPMS-Argonne) and 50 mK base temperature (ii) a cryogen free dilution refrigerator with no applied magnetic field (Blue Fors-Argonne) with a 10 mK base temperature, and (iii) a dilution refrigerator with an 18T superconducting magnet and 20 mK base temperature at the National High magnetic Field Laboratory, Tallahassee (SCM-1, NHMFL-DC

Field). At the NHMFL, we measured the longitudinal ($R_{xx}$) and transverse ($R_{Hall}$) resistances using Lakeshore 372 AC resistance bridges with preamplifiers and a current excitation amplitude well below $I_c$ (typically between 316nA-10 $\mu$A) at frequencies between 9.8-18.2 Hz. All longitudinal resistance data we present is symmetrized $R_{xx} = \frac{R_{xx}(+\mu_0 H)+R_{xx}(-\mu_0 H)}{2}$ and Hall resistance anti-symmetrized $R_{Hall} = \frac{R_{Hall}(+\mu_0 H)-R_{Hall}(-\mu_0 H)}{2}$, after interpolating over an equally spaced interval and FFT smoothing the raw data. We have also accounted for the trapped flux in our low field magnetoresistance measurements. For the displayed data in Table 1 and Fig. 4b, we define the superconducting critical temperature and the upper critical field, $T_c$ and $\mu_0 H_{c2}$, as the midpoint of the resistive transition $R_{xx}(T_c, \mu_0 H_{c2}) = \frac{R_{xx,N}}{2}$. For sample B, we computed $\mu_0 H_{c2}$ from $\frac{1}{2} R_{High\ bias}$ , which is an equivalent definition of $\frac{R_{xx,N}}{2}$, from our differential resistance measurements at base temperature in zero field. We did this because we measured the resistive superconducting transition in a different dilution refrigerator and facility (Blue Fors-Argonne) as the magnetoresistance data (SCM-1, NHMFL-DC Field).

For the differential resistance measurements ($\frac{dV}{dI}$ $vs\ I_{DC}$ in SCM-1, NHMFL-DC Field), we used a Lakeshore 372 AC resistance bridge, for, a SRS CS580 voltage controlled current source, for $I_{DC}$ and a SRS SIM980 summing amplifier to add the signals. We measured the AC voltage drop with the Lakeshore 372. All measured traces were swept from positive DC bias to negative DC bias. Each trace is normalized to 1 by the value at its highest, positive $I_{DC}$ bias $R_{High\text{-}bias}$.

For $R_{xx}$ and $R_{Hall}$ measurements above T = 2 K (PPMS-Argonne), we used lock-in amplifiers with a current excitation amplitude between 1 $\mu$A - 100 $\mu$A at frequencies 177 Hz and 186 Hz. For samples B-F, we measured $R_{xx}$ and $R_{Hall}$ at T=2K, at zero field and $\mu_0$H = 9 T respectively. We computed $n$ and $\mu$ via the Drude model and the sample geometry. For Sample A, we measured $R_{xx}$ and $R_{Hall}$ at T = 2 K, but, as seen in Fig. S2 (b), $R_{Hall}$ is non-linear. Therefore, we performed a linear to fit $R_{Hall}$ and used the slope of $R_{Hall}$ between $\mu_0$H= 5 - 9T as the measure of the Hall carrier density and mobility. Since we only observe a single frequency SdH oscillation, we argue that the non-linearity is due to mobility fluctuations, and not carrier density fluctuations in Sample A. For samples G-J, we measured $R_{Hall}$ using the same methods as samples A-F.

For the cryogen free dilution refrigerator (Blue Fors-Argonne), we used a Lakeshore 372 AC resistance bridge with preamplifiers. We used the cryogen free dilution refrigerator to obtain $R_{xx}(T)$ for samples A, B and C in Fig. 1. We measured the superconducting transitions of samples G-J in this system as well, see Fig. S12.

## Section 3: Electrical transport results

**Resistance measurements above T = 2 K**: All of our samples were metallic down to T=2K, as measured in our PPMS, see Fig. S2 (a). In Fig. S2 (b), we present Hall effect measurements at T=2K.

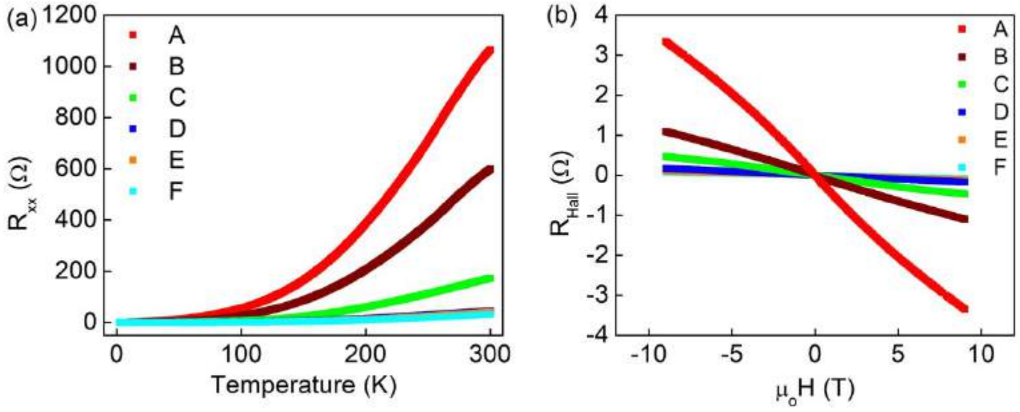


**Fig. S2. Resistance measurements** (a) $R_{xx}$ between T=2K-300K. (b) $R_{Hall}$ at T=2K.

| Sample | $n$ ($10^{17}$ cm$^{-3}$) | $\mu$ (cm$^2$/V-s) | $\rho_N$ (mΩ-cm) | $T_c$ (mK) | $T_{c,0}$ (mK) |
|---|---|---|---|---|---|
| A | 0.385 | 13,712 | 18.63 | 65 | n/a |
| B | 1.03 | 8,594 | 8.10 | 75 | 62 |
| C | 2.40 | 28,978 | 0.63 | 50 | 31 |
| D | 6.59 | 27,100 | 0.45 | 69 | 39 |
| E | 9.89 | 23,520 | 0.26 | 53 | 31 |
| F | 13.68 | 24,143 | 0.24 | 60 | 38 |

**Table S1.** Sample Parameters. $n$ and $\mu$ are the Hall carrier density and mobility respectively. $\rho_N$ is the normal state resistivity. We define $T_c$ at half the normal state resistance and $T_{c,0}$ at zero resistance. The error bars in the $T_c$ phase diagram, Fig. 1 (b), are the transition width defined as: Tc,width=T(0.9$R_N$)-T(0.1$R_N$).

**Low field magnetoresistance measurements**: Magnetoresistance measurements indicating a superconducting state and positive magnetoresistance in modest magnetic fields, both in plane and out of the plane.  All measurements were done on a rotating probe at the base temperature of our dilution refrigerator (SCM-1, NHMFL-DC Field).

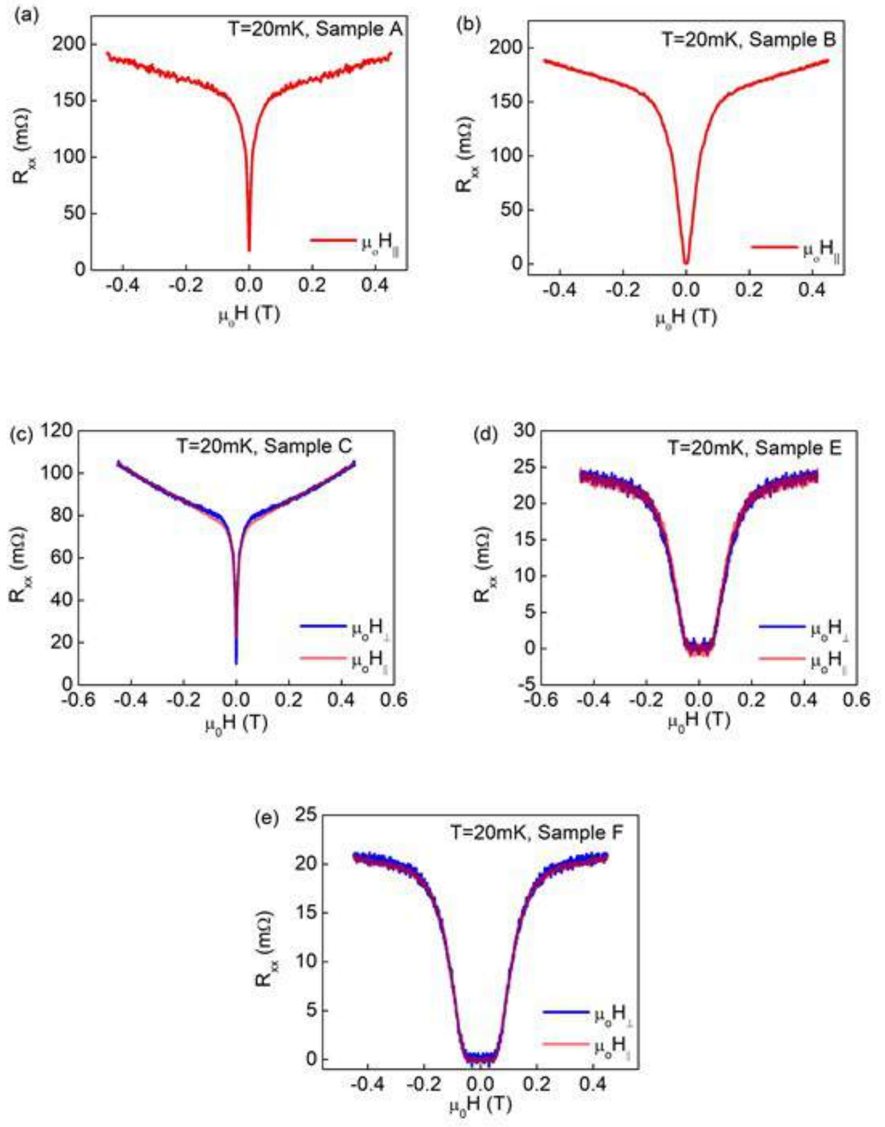


**Fig. S3. (a-d) Low field magnetoresistance plots for samples A,B,C,E,F for out-of-the-plane (black) and in-plane (red) magnetic fields**. **(a)** Sample A shows positive magnetoresistance but no zero-resistance state (as with the measurements in the Blue Fors-Argonne dilution refrigerator). **(b)** Sample B, we observe no in-plane enhancement in the upper critical field (see Fig. S5 for isotropic suppression of superconductivity). In Sample C, the zero-resistance state was not attainable in the setup; however, the positive magnetoresistance associated with the suppression of superconductivity is visible.

**High field magnetoresistance measurements and Shubnikov-de Haas oscillations:** Our high field resistance measurements were out to 18T at the base temperature of our dilution refrigerator (SCM-1, NHMFL-DC Field). After subtracting off a 4$^{th}$ order polynomial fit of the resistance minima, we observe Shubnikov-de Haas oscillations in the magnetoresistance.

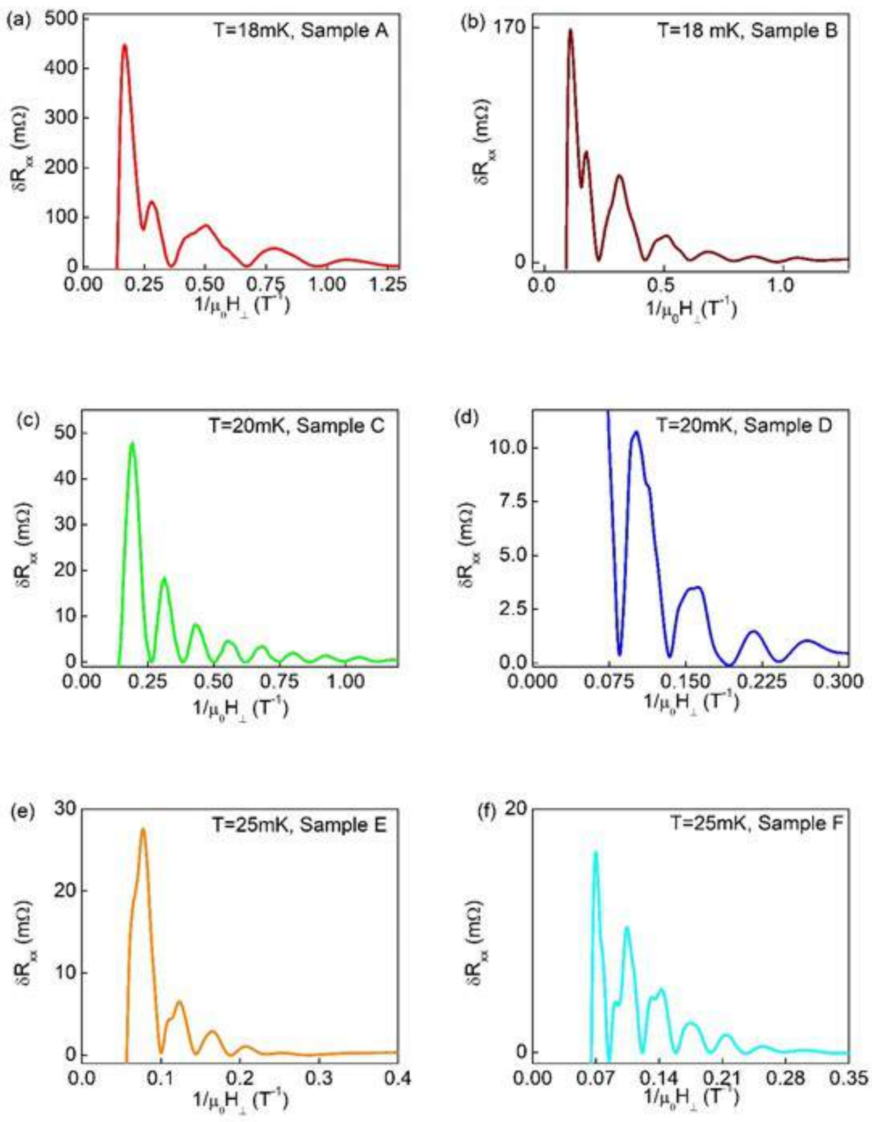


**Fig. S4. (a-e)** $\boldsymbol{\delta R_{xx}\ vs\ {}^{1}/_{\mu_0 H_\perp}}$, Shubnikov de-Haas oscillations in the magnetoresistance for samples A,B,C,D,E,F. The visible peak splitting at low Landau levels is likely due the emergence of spin polarized Landau levels.

| | $n_{Hall}$ $(cm^{-3})$ | $n_{SdH}$ $(cm^{-3})$ | $\Delta n$ (%) |
|---|---|---|---|
| A | 3.85±0.02E16 | 4.86±1.00E16 | 26 |
| B | 1.0266±0.0002E17 | 1.0875±0.3688E17 | 6 |
| C | 2.40±0.02E17 | 1.87±0.13E17 | -22 |
| D | 6.592±0.009E17 | 6.606±1.015E17 | 0.2 |
| E | 9.88±0.04E17 | 8.23 ± 0.55E17 | -17 |
| F | 1.368±0.004E18 | 1.051 ± 0.078E18 | -23 |

**Table S2.** A table of the Hall carrier densities ($n = n_{Hall}$) and SdH carrier densities ($n_{SdH}$), and the discrepancy between these values $\Delta n(\%) = [(n_{SdH} - n_{Hall})/n_{Hall}]$ x 100. Note that the discrepancy $\Delta n$(%) for samples A, B and D are within error bars for $n_{SdH}$.

**Differential resistance measurements:** We used the maxima in $\frac{dV}{dI}$ $vs$ $I_{DC}$ to determine $I_c$.

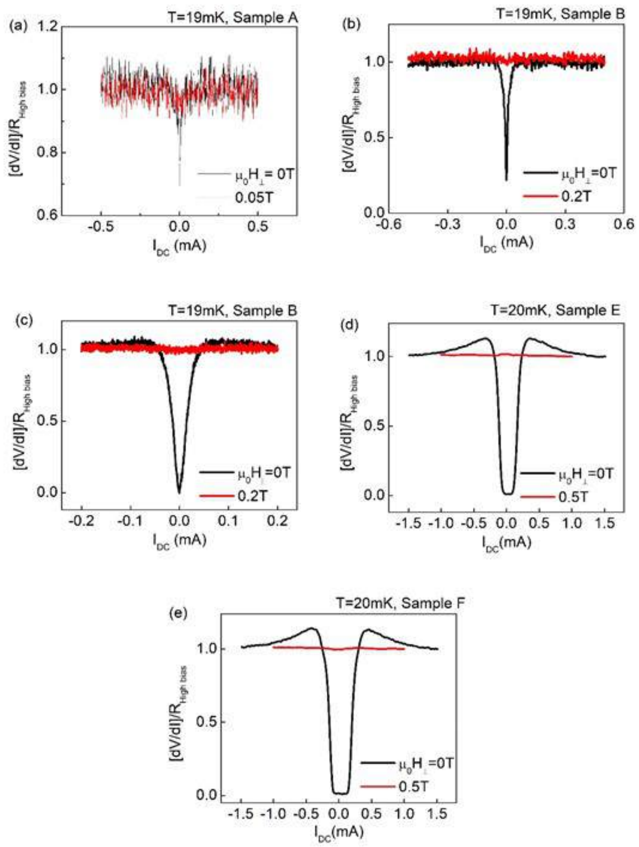


**Fig. S5. (a)** Sample A, **(b,c)** B **(d)** E **(e)** F. Note the complete isotropic suppression of the supercurrent with an application of the magnetic field ($\mu_0$H=0.2T) like the other samples. All of the traces have been normalized to their value at the highest, positive $I_{DC}$ bias ($R_{High\ bias}$).

## Section 4: Tunnel diode oscillator (TDO) results

**TDO measurements on Sample E and LuPdBi:** The TDO measurements on sample E and the LuPdBi single crystal were comprised of the same RF electronics and heterodyning technique.

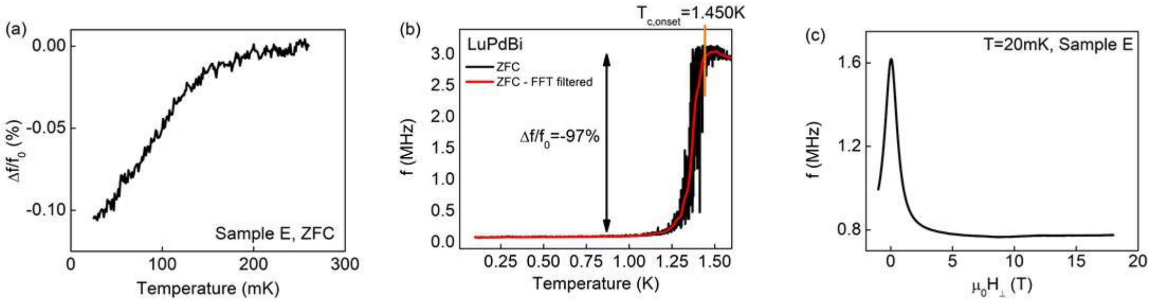


**Fig. S6. (a,c)** $\frac{\Delta f(T)}{f_0}$ resonant frequency shift of the TDO circuit for sample E. **(b)** The resonant frequency of the TDO circuit on a noncentrosymmetric, low carrier density superconductor LuPdBi single crystal. We show the measured resonant frequency in black and the resonant frequency with an FFT filter as a guide. In **(a)**, there is no indication of a superconducting transition ($\frac{\Delta f}{f_0} \sim -0.1\%$) while in **(b)** there is an enormous frequency shift ($\frac{\Delta f}{f_0} \sim -97\%$) indicating a superconducting transition with a $T_{c,onset} = 1.45K$. In **(c)**, we observe the changes in the resonant frequency of the TDO circuit as a function of magnetic field for sample E. In this case, changes in $f$ are due to the magnetoresistance of the circuit components and the STO in the normal state.

## Section 5: Computed length and energy scales and estimates of the depairing currents

**Normal state and superconducting length scales:** In the spirit of X. Lin, Z. Zhu, B. Fauqué, and K. Behnia, Phys. Rev. X 3, 021002 (2013), we computed relevant normal state and superconducting length scales, for samples A-F, as an additional check to determine whether or not our samples were metallic ($\lambda_F < l_{elastic}$) and within the BCS limit ($d_{interelectron} < \xi_{BCS}$). Additionally, we estimate the London penetration depth and $\Delta/_{k_B T_c}$ for samples A-F.

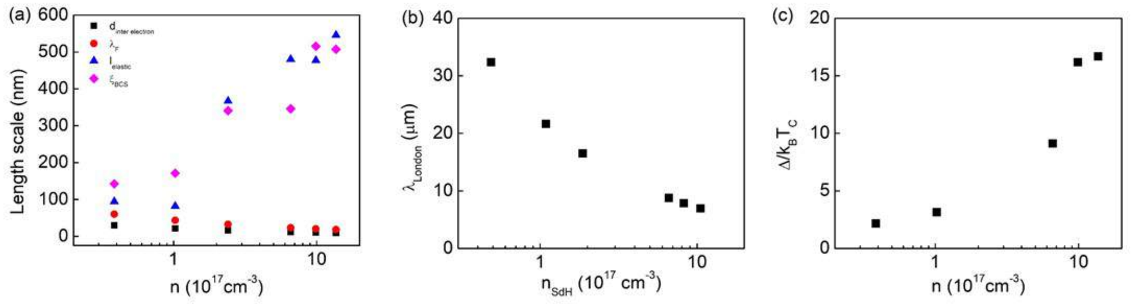


**Fig. S7. (a,b)** A semi-log plots of normal state and superconducting length scales for samples A-F. The normal state length scales (interelectron spacing - $d_{interelectron}$, the Fermi wavelength - $\lambda_F$ and elastic mean free path-$l_{elastic}$) were computed from the longitudinal and Hall resistances at T=2K using the Drude model and an effective mass of $1.8m_e$ . We computed $\xi_{BCS}$ from $\xi_{BCS} = \frac{\hbar v_F}{\pi\Delta(0)}$ , $v_F$ from the Hall measurements of $n$ and $\Delta(0) = 1.76k_B T_c$. As seen here, our samples are metallic ($\lambda_F < l_{elastic}$) and with the computed size of the Cooper pairs being larger than the interlectron spacing ($d_{interelectron} < \xi_{BCS}$). **(b)** A simple estimate for the London penetration depth as a function of $n_{SdH}$. This uses $\lambda_{London} = \left(\frac{m^* c^2}{4\pi n_s q^2}\right)^{1/2}$, with $m^* = 2 * 1.8m_e$, $n_s = \frac{n_{SdH}}{2}$ and $q = 2e$. **(c)** $\Delta/_{k_B T_c}$ vs. $n$ where we estimate $\Delta \approx \hbar v_F/_{\pi\xi}$ with $\xi = \sqrt{\Phi_0/_{2\pi\mu_0 H_{c2}}}$ from our $\mu_0 H_{c2}$ data.

**Estimated depairing current density:** We use $J_{depairing} = 2en_s v_c;\ v_c = \frac{\Delta(0)}{\hbar k_F}$ and $n_s = \frac{n}{2}$.[1]

| | $J_c$ (mA/cm$^2$) | $J_{depairing}$ (mA/cm$^2$) | Ratio ($J_{depairing}$/Jc) |
|---|---|---|---|
| A | 2.8 | 88,635 | 31,655 |
| B | 7 | 196,555 | 28,079 |
| D | 31.7 | 624,741 | 19,708 |
| E | 26 | 569,488 | 21,903 |
| F | 36 | 883,867 | 24,552 |

**Table S3.** Measured critical current densities ($J_c$) and depairing current densities ($J_{depairing}$).

## Section 6: Paraconductivity and EMT fits, theoretical discussions

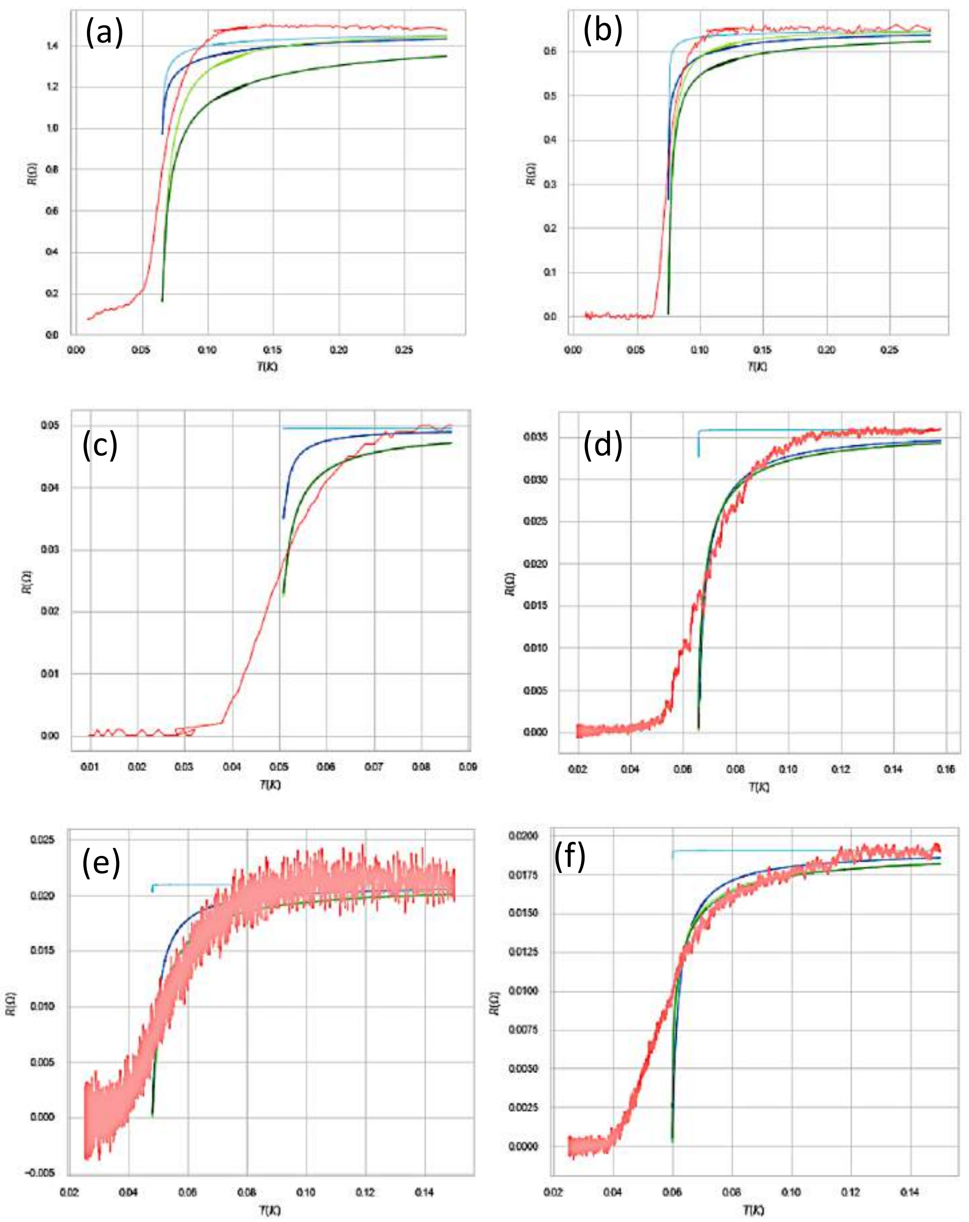


**Fig. S8. Paraconductivity fits (a-f)** to samples A-F. Light blue: homogeneous 3D; dark blue: percolative 3D; light green: homogeneous 2D; dark green: percolative 2D.

| | $n$ ($10^{17}$ $cm^{-3}$) | $\xi$ measured (nm) | $d$ homogeneous (nm) | $d$ percolative (nm) | $\xi_p$ 3D (µm) | $\xi_p$ 2D (µm) |
|---|---|---|---|---|---|---|
| A | 0.385 | 26 | 26 | 26 | .026 | .026 |
| B | 1.0266 | 27 | 27 | 27 | .067 | .027 |
| C | 2.40 | 690 | 38 | 140 | 69 | 11 |
| D | 6.593 | 63 | 14 | 40 | 4.1 | .66 |
| E | 9.89 | 57 | 27 | 31 | 5.7 | 1.3 |
| F | 13.68 | 54 | 4.1 | 8.9 | 4.7 | .25 |

**Table S4.** Fitting parameters of experimental data to paraconductivity models. ξ the superconducting coherence length, $\xi_p$ is the characteristic percolative length, and d is the thickness of a 2d superconducting region.

**Theoretical discussion and details of the paraconductivity fits**

As $T_C$ is approached from above, pairing fluctuations give rise to short-lived Cooper pairs which provide an additional channel for charge transport before decaying. Formally, their contribution may be calculated by expanding the Ginzburg-Landau free energy functional in $\varepsilon = (T-T_C)/T_C$, but to leading order it turns out to be adequate to use a Drude-like formula for the excess conductivity, with the Cooper pair density of states $\langle|\psi_q|\rangle \propto kT/(1+\xi(T)^2q^2)$ and relaxation time obtained from the Ginzburg-Landau calculation. This produces the Aslamasov-Larkin (AL) term

$$\sigma_{AL} = \frac{e^2}{\hbar}\begin{cases} \dfrac{1}{32\,\xi(0)}\varepsilon^{-1/2} & 3D \\ \dfrac{1}{16\,d}\varepsilon^{-1} & 2D \end{cases}$$

A second contribution comes from the tendency of unpaired electrons of small total momentum undergoing diffusive motion to scatter into a paired state. In three dimensions this term ends up functionally identical to the AL term, but in two dimensions and below, where the return probability for diffusion becomes unity, it is divergent unless cut off by some intrinsic microscopic pair-breaking process which, in analogy to a pair-breaking magnetic field will produce a shift in $T_C$, parameterized by $\delta=(T_{C0}-T_C)/T_C$. In 2D this Maki-Thompson (MT) contribution assumes the form

$$\sigma_{MT} = \sigma_{AL}\frac{2\varepsilon}{\varepsilon-\delta}\ln\frac{\varepsilon}{\delta}$$

and diverges even more strongly in 1D. The total conductivity is then $\sigma=\sigma_N+\sigma_{AL+}\sigma_{MT}$, where $\sigma_N$ is the normal-state conductance. We note in passing that for the wide transitions measured and these low transition temperatures, ε is not strictly small and the power law derived from expanding in ε is no longer valid, as fluctuations begin to decay logarithmically at higher temperatures [2].

We begin by fitting the resistance data to the 2D and 3D paraconductivity expressions above. In 3D the only parameter is ξ and we plot using the measured value, whereas in 2D our fitting parameters are d and δ. The lines of best fit are shown in Fig. S8 (a)-(f) and the extracted parameters are in Table S4.

The homogeneous 3D expression substantially underestimates the width of the transition in all samples. In 2D, the inferred thickness of the superconducting region is plausible, of order nm and smaller than the measured coherence length, except for the two most dilute samples, where it saturates at the maximum physical value, d=ξ. Interestingly it is these samples that are least poorly described by the 3D theory, suggesting a possible dimensional crossover such as is seen in layered high-$T_C$ materials.

As it is clear that superconductivity is not confined to a single layer of thickness *d*, due to the isotropic behavior with respect to rotating the magnetic field, and because at the same time we see such anomalously low critical currents that suggest weak links, we look for a model that takes into account the putative inhomogeneity of the system. We adopt the percolative model of Char and Kapitulnik. Physically, it assumes that the material consists of some distribution of regions, some fraction of which go superconducting, and that the superconducting transition is achieved by establishing a supercurrent path connecting these regions. At long wavelengths, fluctuations explore the physical dimension of the sample. At shorter wavelengths, however, their excursions are constrained by the geometry of the percolation network. In particular, within a percolation correlation length $\xi_p$ determined by proximity to the percolation threshold, the network is self-similar with a fractal dimension of 4/3. Therefore in this model there is a set of fluctuations, whose relative importance is controlled by $\xi_p/\xi$, which always reside in a lower spatial dimension and therefore contribute both an AL with a steeper power law, and a more strongly divergent MT term.

To give some intuition for the behavior of these models, we plot in Fig. S9 families of curves for the percolative 3D model and the homogeneous 2D model. The former has a wider power law but the overall magnitude of the fluctuations is still set by ξ, whereas in the latter, the thickness d scales the magnitude of the paraconductivity.

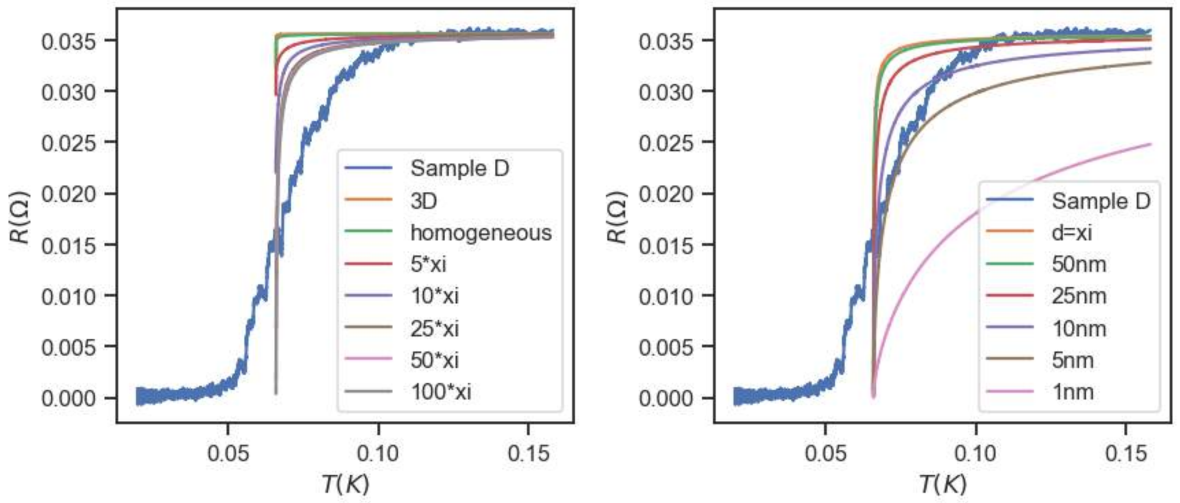


**Fig. S9. Behavior of paraconductivity models** Left: percolative 3D for different $\xi_p$; right: homogeneous 2D for different d. In both curves, δ=.01.

The model contains a number of possible crossover parameters, which we set to unity to avoid overfitting. In these fits we again choose to constrain ξ to the measured value, so we are left with $\xi_p$, δ, and d free. The fits are again displayed in Fig. S8 (a)-(f) and the parameters in Table S3. We emphasize that in any case quantitative agreement with the data has not been achieved, and indeed the qualitative improvement over a homogeneous model is not always noticeable by eye. Generally, the 2D fits find d ~ ξ/10 and $\xi_p$ ~ 10 ξ, except in the more dilute samples, which although poorly described by the homogeneous 3D theory do not do much better in lower dimensions. The tension that leads to qualitative disagreement with the data is between the broad transition in the vicinity of $T_C$, and the rapid approach to $R_N$ at higher temperatures, which in fact is faster than power-law.

Let us briefly note some reasons that quantitative agreement is not expected. 1. As mentioned, ε is not small. 2. We expect to have a distribution of $T_C$ in the various regions, and therefore as the temperature is lowered, $\xi_p$ should change. 3. We have not considered possible dimensional crossovers. 4. A true microscopic theory that accounts for the distribution of superconducting regions in the sample is likely to be constrained beyond a simple percolation model.

**Effective Medium Theory**

To capture the effects of a distribution of $T_c$, we employ the same effective medium theory (EMT) used in [3]. The EMT provides a mean-field solution to a resistor network problem, where each resistor represents a mean-field description of some superconducting region. The properties of the network, including dimensionality, are represented a percolation threshold $p_c$, which we take to be $p_c \approx .3$ for simple cubic site percolation, although at this level of analysis there is only a small

quantitative difference. The $T_c$ of each resistor is drawn from a Gaussian distribution p(T) characterized by a mean and variance, and the superconducting fraction f is the survival function of this distribution. The conductivity σ in units of the normal-state conductivity is then given by the solution of

$$\frac{\sigma-(1-f+f/\varepsilon)}{1-f+f/\varepsilon+(p_c-1)\sigma}f+\frac{\sigma-\dfrac{1/\varepsilon}{f-(1-f)/\varepsilon}}{f+(1-f)/\varepsilon\;+(1/p_c-1)\sigma}(1-f)=0$$

where ε is the vanishing resistance of a superconducting patch. In Fig. S10 we plot the data alongside this model's resistance for representative choices of p(T), and in Fig. S11 we plot the mean $T_C$ and variance that best characterize the data at each density. Notably, the mean $T_C$ of the distribution is generally substantially lower than $T_C$ defined by $R_N/2$, but this can largely be tuned by selecting a different $p_c$ and should not be taken seriously absent a microscopic model of the domain geometry.

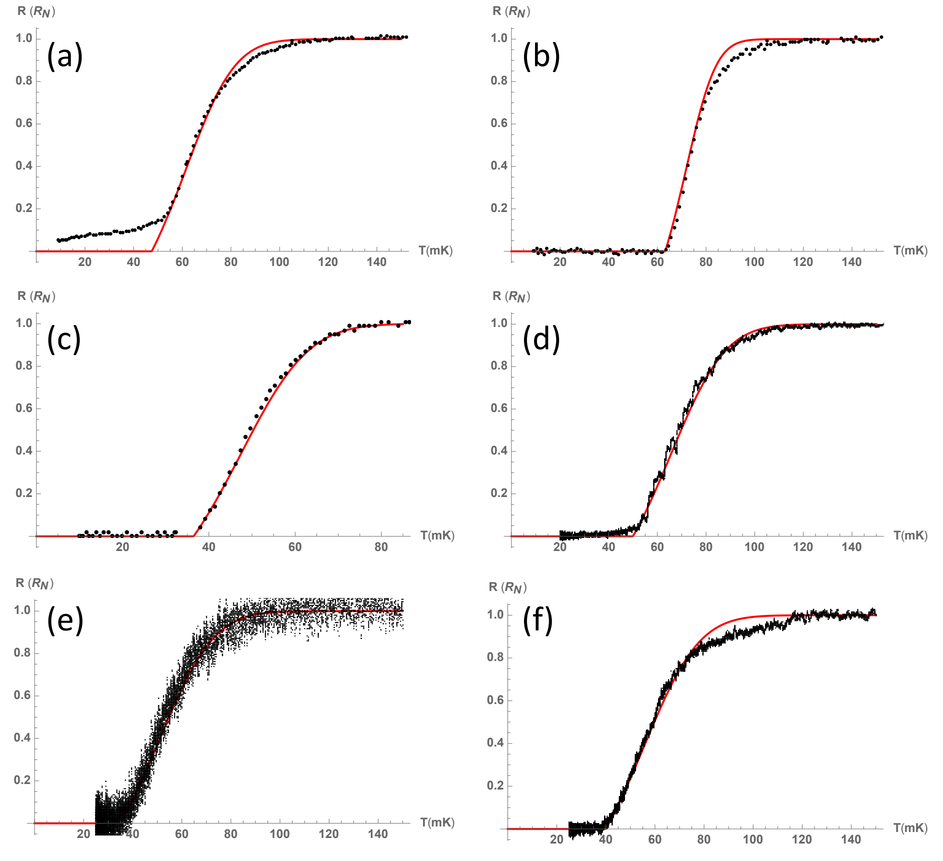


**Fig. S10. EMT fits (a-f)** to samples A-F.

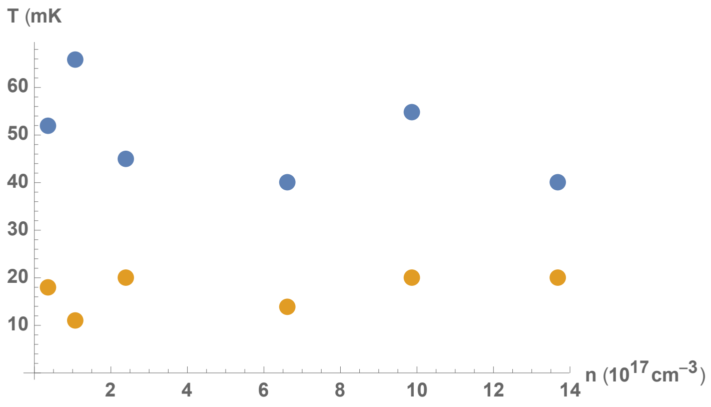


**Fig. S11.** EMT distribution parameters for fits to samples A-F. Mean $T_C$ in blue and standard deviation in orange.

## Section 7: Superconducting transitions for samples G-J (measured along [011])

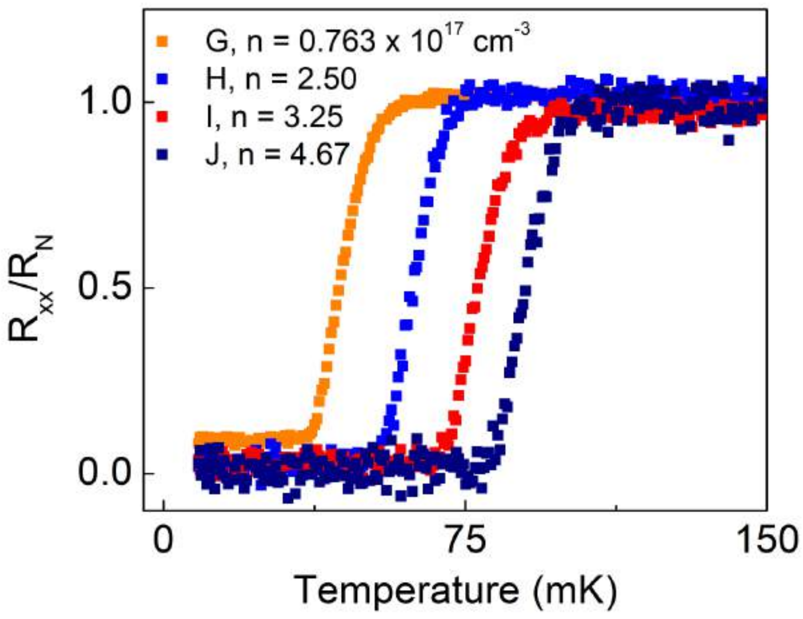


**Fig. S12.** The resistive superconducting transitions for samples G-J. Transport is along the [011] crystallographic axis.

[1] M. Tinkham, Introduction to Superconductivity, Second Edition, Dover Publications, Inc., Mineola, NY (2004).
[2] L. G. Aslamasov and A. A. Varlamov, J Low Temp Phys **38**, 223 (1980).
[3] P. Popčević, D. Pelc, Y. Tang, K. Velebit, Z. Anderson, V. Nagarajan, G. Yu, M. Požek, N. Barišić, and M. Greven, Npj Quant Mater 3, 42 (2018).
